# Supplementary material for: Towards Gradient-based Time-Series Explanations through a SpatioTemporal Attention Network
Source: arXiv:2405.17444 source file (2024-05-18)
Supplement: Supplementary file 1 [file appendix.tex]

\appendix
